# Supplementary material for: Detection of concealed cars in complex cargo X-ray imagery using Deep Learning
Source: arXiv:1606.08078 ancillary file (2016-09-09)
Supplement: Supplementary file 1 [file CNN_Architecture_Details.pdf]

## 1. Supplementary material

Table 1: 11-layer CNN architecture, adapted from [42]. For convolution networks, $r$ denotes the dimensions of the receptive field, $c$ the number of channels, and $p$ the padding. Rectified linearity units are not shown for clarity.

| Layer | Input dim. | Output dim. |
|---|---|---|
| Convolutional ($r = 3 \times 3$, $c = 64$, $p = 1$) | $256 \times 256 \times 1$ | $256 \times 256 \times 64$ |
| Max pooling ($2 \times 2$) | $256 \times 256 \times 64$ | $128 \times 128 \times 64$ |
| Convolutional ($r = 3 \times 3$, $c = 128$, $p = 1$) | $128 \times 128 \times 64$ | $128 \times 128 \times 128$ |
| Max pooling ($2 \times 2$) | $128 \times 128 \times 128$ | $64 \times 64 \times 128$ |
| Convolutional ($r = 3 \times 3$, $c = 256$, $p = 1$) | $64 \times 64 \times 128$ | $64 \times 64 \times 256$ |
| Convolutional ($r = 3 \times 3$, $c = 256$, $p = 1$) | $64 \times 64 \times 256$ | $64 \times 64 \times 256$ |
| Max pooling ($2 \times 2$) | $64 \times 64 \times 256$ | $32 \times 32 \times 256$ |
| Convolutional ($r = 3 \times 3$, $c = 512$, $p = 1$) | $32 \times 32 \times 256$ | $32 \times 32 \times 512$ |
| Convolutional ($r = 3 \times 3$, $c = 512$, $p = 1$) | $32 \times 32 \times 512$ | $32 \times 32 \times 512$ |
| Max pooling ($2 \times 2$) | $32 \times 32 \times 512$ | $16 \times 16 \times 512$ |
| Convolutional ($r = 3 \times 3$, $c = 512$, $p = 1$) | $16 \times 16 \times 512$ | $32 \times 32 \times 512$ |
| Convolutional ($r = 3 \times 3$, $c = 512$, $p = 1$) | $16 \times 16 \times 512$ | $32 \times 32 \times 512$ |
| Max pooling ($2 \times 2$) | $8 \times 8 \times 512$ | $4 \times 4 \times 512$ |
| Fully-connected ($r = 4 \times 4$, $c = 4096$) | $4 \times 4 \times 512$ | $1 \times 1 \times 4096$ |
| Fully-connected ($r = 1 \times 1$, $c = 4096$) | $1 \times 1 \times 4096$ | $1 \times 1 \times 4096$ |
| Fully-connected ($r = 1 \times 1$, $c = 2$) | $1 \times 1 \times 4096$ | $1 \times 1 \times 2$ |
| Softmax | $1 \times 1 \times 2$ | $1 \times 1 \times 1$ |

Table 2: 19-layer CNN architecture, adapted from [42]. For convolution networks, $r$ denotes the dimensions of the receptive field, $c$ the number of channels, and $p$ the padding.Rectified linearity units are not shown for clarity.

| Layer | Input dim. | Output dim. |
|---|---|---|
| Convolutional ($r = 3 \times 3$, $c = 64$, $p = 1$) | $256 \times 256 \times 1$ | $256 \times 256 \times 64$ |
| Convolutional ($r = 3 \times 3$, $c = 64$, $p = 1$) | $256 \times 256 \times 64$ | $256 \times 256 \times 64$ |
| Max pooling ($2 \times 2$) | $256 \times 256 \times 64$ | $128 \times 128 \times 64$ |
| Convolutional ($r = 3 \times 3$, $c = 128$, $p = 1$) | $128 \times 128 \times 64$ | $128 \times 128 \times 128$ |
| Convolutional ($r = 3 \times 3$, $c = 128$, $p = 1$) | $128 \times 128 \times 128$ | $128 \times 128 \times 128$ |
| Max pooling ($2 \times 2$) | $128 \times 128 \times 64$ | $64 \times 64 \times 128$ |
| Convolutional ($r = 3 \times 3$, $c = 256$, $p = 1$) | $64 \times 64 \times 128$ | $64 \times 64 \times 256$ |
| Convolutional ($r = 3 \times 3$, $c = 256$, $p = 1$) | $64 \times 64 \times 256$ | $64 \times 64 \times 256$ |
| Convolutional ($r = 3 \times 3$, $c = 256$, $p = 1$) | $64 \times 64 \times 256$ | $64 \times 64 \times 256$ |
| Max pooling ($2 \times 2$) | $64 \times 64 \times 64$ | $32 \times 32 \times 256$ |
| Convolutional ($r = 3 \times 3$, $c = 512$, $p = 1$) | $32 \times 32 \times 256$ | $32 \times 32 \times 512$ |
| Convolutional ($r = 3 \times 3$, $c = 512$, $p = 1$) | $32 \times 32 \times 512$ | $32 \times 32 \times 512$ |
| Convolutional ($r = 3 \times 3$, $c = 512$, $p = 1$) | $32 \times 32 \times 512$ | $32 \times 32 \times 512$ |
| Max pooling ($2 \times 2$) | $32 \times 32 \times 256$ | $16 \times 16 \times 512$ |
| Convolutional ($r = 3 \times 3$, $c = 512$, $p = 1$) | $16 \times 16 \times 512$ | $16 \times 16 \times 512$ |
| Convolutional ($r = 3 \times 3$, $c = 512$, $p = 1$) | $16 \times 16 \times 512$ | $16 \times 16 \times 512$ |
| Convolutional ($r = 3 \times 3$, $c = 512$, $p = 1$) | $16 \times 16 \times 512$ | $16 \times 16 \times 512$ |
| Max pooling ($2 \times 2$) | $16 \times 16 \times 512$ | $8 \times 8 \times 512$ |
| Convolutional ($r = 3 \times 3$, $c = 512$, $p = 1$) | $8 \times 8 \times 512$ | $8 \times 8 \times 512$ |
| Convolutional ($r = 3 \times 3$, $c = 512$, $p = 1$) | $8 \times 8 \times 512$ | $8 \times 8 \times 512$ |
| Convolutional ($r = 3 \times 3$, $c = 512$, $p = 1$) | $8 \times 8 \times 512$ | $8 \times 8 \times 512$ |
| Max pooling ($2 \times 2$) | $8 \times 8 \times 512$ | $4 \times 4 \times 512$ |
| Fully-connected ($r = 4 \times 4$, $c = 4096$) | $4 \times 4 \times 512$ | $1 \times 1 \times 4096$ |
| Fully-connected ($r = 1 \times 1$, $c = 4096$) | $1 \times 1 \times 4096$ | $1 \times 1 \times 4096$ |
| Fully-connected ($r = 1 \times 1$, $c = 2$) | $1 \times 1 \times 4096$ | $1 \times 1 \times 2$ |
| Softmax | $1 \times 1 \times 2$ | $1 \times 1 \times 1$ |
